# Supplementary material for: Concept Activation Regions: A Generalized Framework For Concept-Based Explanations
Source: arXiv:2209.11222 source file (2022-09-29)
Supplement: Supplementary file 1 [file car_supp.tex]

\textbf{More than one concept.} Now that we are equipped with a principled way of extracting a CAR $\H^c$ for each concept $c \in [C]$, let us discuss the situation where we manipulate more than one concept at-a-time. Let us assume that we are given an example $\x \in \X$ whose representation lies in more than one CAR: $\g(\x) \in \bigcap_{c \in \C_{\x} \subseteq [C]} \H^c$. This tells us that the concepts $\C_{\x} \subset [C]$ are relevant for the black-box to represent $\x$. Now we might want to rank these concepts according to how relevant they are. In the CAV formalism, this is achieved by analyzing the concept sensitivities $S^c_k(\x)$ for the various concepts $c \in \C_{\x}$ where $k \in [d_Y]$ is the class associated to $\x$. In the CAR formalism, it is not clear how to choose a CAV for the computation of these sensitivities. For this reason, we use the concept densities $\rho^c(\x)$ directly in order to estimate the relative importance of each concept. In this way, sorting the densities $\{ \rho^c[\g(\x)] \mid c \in \C_{\x}\}$ in decreasing order is equivalent to sorting the concepts in decreasing order of importance. The rationale behind this approach is the following: if we have $\rho^{c_1}[\g(\x)] > \rho^{c_2}[\g(\x)]$ indicates that the representation $\g(\x)$ is located of a region of the latent space where positive examples for $c_1$ are closer than those of $c_2$. If we follow Assumption~\ref{assumption:smoothness}, this leads us to believe that $c_1$ is more salient than $c_2$ in building the representation for $\x$. We note that, in contrast with the concept sensitivity $S^c_k(\x)$, the density $\rho^c(\x)$ is \emph{intrinsic} to the representation space $\H$. This means that neither the map $\l$ nor a label $k \in [d_Y]$ are required to evaluate the density. This is particularly interesting if we are trying to interpret unsupervised models or examples for which no ground-truth label is available~\cite{Crabbe2022}. We now proceed to show how the density allows us to define concept-based feature importance.

It is possible to define a similar score to estimate how the model relates two concepts with each other. We define the TCAR score associated to the concepts $c_1, c_2 \in [C]$ as the ratio $\TCAR^{c_1, c_2} = \nicefrac{\card{\g(\D) \bigcap \H^{c_1} \bigcap \H^{c_2} }}{\card{\g(\D) \bigcap (\H^{c_1} \bigcup \H^{c_2})}}$. Again, $\TCAR = 0$ corresponds to no overlap and $\TCAR = 1$ describes a perfect overlap.
